# Supplementary material for: PIV3CAMS: a multi-camera dataset for multiple computer vision problems and its application to novel view-point synthesis
Source: arXiv:2407.18695 source file (2024-07-26)
Supplement: Supplementary file 1 [file Appendix.tex]

\appendix
\chapter{First Appendix Chapter Title}
